# Supplementary material for: Alignment Based Matching Networks for One-Shot Classification and Open-Set Recognition
Source: arXiv:1903.06538 source file (2019-03-11)
Supplement: Supplementary file 1 [file supp.tex]

\clearpage
\section{Supplementary Information}

\begin{figure}[h]
  \centering
  \begin{tabular}{cccccccccccc}
    &$T_1$&$S_1$&$P_1$& &$T_2$&$S_2$&$P_2$& &$T_3$&$S_3$&$P_3$
  \end{tabular}

    \includegraphics[width=0.5\textwidth]{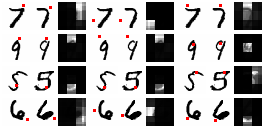}
        \begin{tabular}{c}
  \hline
  \hline
  \end{tabular}
    \includegraphics[width=0.5\textwidth]{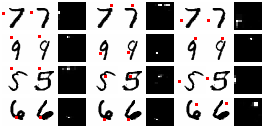}
  \caption{Three points sampled uniformly from the test image ($T_1=T_2=T_3$) are mapped to the reference image ($S_1=S_2=S_3$). The red point in the test image is the point selected for matching. The red point in  the reference image shows the corresponding minimum cost matching. The matching probability ($P_1, P_2, P_3$) is obtained by matching the selected point to all points in the reference image. Each row show a  different test-reference image pair. Results are shown for ABM Nets without (top) and with (bottom) self-regularization}
  \label{fig:mnistPointMatch}
\end{figure}

\begin{figure}
  \centering
  \begin{tabular}{cccccccccccc}
    &$T_1$&$S_1$&$P_1$& &$T_2$&$S_2$&$P_2$& &$T_3$&$S_3$&$P_3$
  \end{tabular}

    \includegraphics[width=0.5\textwidth]{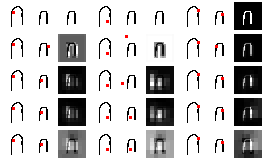}

  \caption{Exploring the effect of hyper-column filters on the point matching distribution. The first row uses only the highest resolution filters thereby aligning only based on pixel color. Adding in filters from increasingly coarser layers helps discriminate which area of the image the point lies in. Three points are sampled uniformly from the test image ($T_1=T_2=T_3$) are mapped to the reference image ($S_1=S_2=S_3$). The red point in the test image is the point selected for matching. The red point in  the reference image shows the corresponding minimum cost matching. The matching probability ($P_1, P_2, P_3$) is obtained by matching the selected point to all points in the reference image.}

  \label{fig:pointMaskCost1}
\end{figure}

\begin{figure}
  \centering
  \begin{tabular}{cccccccccccc}
    &$T_1$&$S_1$&$P_1$& &$T_2$&$S_2$&$P_2$& &$T_3$&$S_3$&$P_3$
  \end{tabular}

    \includegraphics[width=0.5\textwidth]{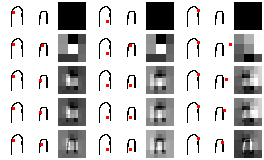}

  \caption{Exploring the effect of hyper-column filters on the point matching distribution. The first row uses only the coarsest filters and is unable to localize the point (uniform probability across all pixels). As we add in filters from increasingly finer layers, we see that the model is able to better localize the point in the image.}

  \label{fig:pointMaskCost2}
\end{figure}
